# Supplementary material for: Aligning Autoresearch: Co-Improvement between Agents and Humans
Source: arXiv:2610.38882 source file (2026-10-28)
Supplement: Supplementary file 1 [file metarubric_appendix.tex]

One meta-prompt is used for \emph{both} rubric variants; the optimizer produces a
single template per iteration. Blind vs.\ GT-informed generation is not a difference
in instructions but in what is substituted for the \texttt{\{paper\}} slot: the blind
variant receives the paper with the target section removed, while the GT-informed
variant receives the same text with the held-out human section appended under a
header
\begin{center}\texttt{----- ACTUAL <SECTION> (ground truth) -----}\end{center}
so the generator reads identical instructions and only differs in whether it can see
the section it is writing a rubric for. Below is the final meta-prompt (iteration~3),
shown as the \texttt{.format()} template with \texttt{\{section\_label\}},
\texttt{\{target\_words\}}, and \texttt{\{paper\}} left as placeholders.

\begin{lstlisting}
You are an expert reviewer for a top ML/CS venue. You will be shown a paper and must design a RUBRIC for grading a candidate writing of its {section_label} (target length: {target_words} words).

The rubric is applied blind to several candidates: one is the paper's real, published {section_label}; the others are machine imitations written by a model that has also read the whole paper. A GOOD rubric ranks the expert human writing first, for the right reasons. Rubrics have been failing at this in three specific, diagnosable ways. Your entire job is to design against all three.

FAILURE 1 --- THE SUPERSET CHECKLIST. Because you can see the whole paper, it is tempting to name its facts (a mechanism, a lineage, a metric, a benchmark, a secondary technique) and ask whether the candidate "covers" them. The imitation harvests details from every part of the paper and packs them in, so it will win any coverage contest. In past runs, almost every under-scored human section was marked down with a note of the form "omits X, Y, and Z" --- where X, Y, Z were deliberate editorial cuts, and the model's inclusion of them was indiscriminate dumping. Therefore: your criteria must never make presence of a specific fact a scoring condition. Name concrete paper facts ONLY inside "this is a liability here / do not require this" lists --- never inside "should mention" lists.

FAILURE 2 --- REWARDING SCAFFOLDED POLISH. Model prose looks good at a glance: a thesis announced in sentence one, uniformly shaped paragraphs, a "however, this leaves a gap" clause closing each one, tricolons, "Critically/Notably/Importantly", a final sentence restating the contribution a third time. Human expert prose is less symmetric, leaves some connections implicit, and carries positioning inside precise technical clauses instead of announcement sentences. A rubric that rewards visible signposting rewards the imitation.

FAILURE 3 --- MISTAKING DENSITY FOR QUALITY. This is the dominant recent failure. Graders wrote notes like "technically precise and faithful, excellent alignment --- the only problem is the dataset and baseline enumeration," and then scored that candidate ABOVE a clean, well-judged human section. Packed inventories of numbers, model names, datasets, losses, and training details are not "precision plus a minor scope issue"; in a section that should not carry them they are the primary defect, and they must dominate the score. Your rubric must be built so that a candidate whose faults are "over-inclusion, re-narration, extra specifics" cannot outscore a candidate whose faults are "left some available detail out."

THE ONE JOB OF THIS SECTION

Decide the single rhetorical job {section_label} does in THIS paper and grade whether the candidate does that job with well-chosen material, not whether it recites the paper.
- abstract: one self-contained arc (problem -> what the status quo cannot do -> what we do -> what it buys), carrying only the evidence the claim needs. Baseline lists, dataset inventories, exact per-benchmark numbers, counts, hyperparameters, architecture internals are liabilities.
- introduction: motivation, a sharp gap, the key idea stated as an idea, contributions that follow from it. Headline-level evidence only; no protocol, ablation menus, equations, module names doing the work of an explanation.
- related work: prior work positioned against this paper with correct, specific attribution. Positioning may be carried implicitly by precise technical description; an explicit gap paragraph is optional and manufactured themes are a defect. Internals of this paper's method, its equations, its results, and its contribution claims are severe violations here.
- conclusion: synthesis and perspective --- what was learned, why it matters, what the honest scope is. Re-narrating setup, benchmark names, metrics, and numbers makes a conclusion worse. Never require a limitations sentence as a checkbox.

CONSTRUCTION RULES (hard)

1. Write 4 to 6 criteria, float weights summing to 1.0.

2. AT MOST ONE argument criterion, weight <= 0.20. Frame it as argument integrity, not coverage: "does the candidate make a coherent, self-sufficient version of the claim this section exists to make, and is that claim true of this paper?" It must state that any economical route to the argument earns full credit; that a candidate which selects a different but coherent subset of the paper's material earns full credit; and that a grader may deduct for an absent item ONLY if they can state in one sentence how the argument becomes false, unsupported, or incoherent without it. Vague dissatisfaction ("does not mention the mechanism") is not a valid deduction. Do not enumerate required content.

3. The remaining >= 0.80 goes to craft, discipline, and integrity criteria, each made concrete to this paper's material:
   - Necessity and scope discipline (weight 0.30--0.35, the largest single criterion). Ask: is anything here material this section should not carry? List, using this paper's actual specifics, the concrete over-inclusions you expect (e.g. the named datasets, the baseline set, the exact headline numbers, the loss terms, the optimizer/schedule, the module names, the ablation framing, this paper's method internals if the section is related work). Give an explicit schedule: full credit only if essentially every sentence is load-bearing for this section's job; deduct roughly one point per distinct unnecessary specific or re-narrated passage; three or more such intrusions, or any passage that reads as an inventory, caps this criterion in its lower third regardless of fluency or accuracy. State plainly that a shorter section that leaves out available detail is exhibiting judgment, not deficiency, and that breadth never compensates for a scope violation.
   - Economy, authorial control, and non-formulaic prose (0.20--0.25). Reward sentences that are technically exact and subordinate detail to claims (main clause carries the point; specifics live in modifiers), varied paragraph shapes, transitions expressing real logical relations, and commitment instead of hedging. Penalize: restating the same point a second or third time, template scaffolding (thesis announcements, paragraph-final gap declarations, "Moreover/Additionally/Furthermore" chains), hollow intensifiers ("significant", "crucial", "comprehensive", "state-of-the-art"), promotional framing, vacuous openers, and telegraphic fact-strings where a sentence merely concatenates specifics. State explicitly that packed factual density is not economy: a paragraph that is dense with material this section should not carry scores worse than a plainer paragraph that carries only what is needed. Weigh systematic scaffolding more heavily than an isolated stock transition.
   - Faithfulness, attribution, and calibration (0.20, strict). Name one or two concrete ways a candidate could get THIS paper's facts subtly wrong: a number attributed to the wrong configuration or backbone, a mechanism described as doing something adjacent to what it does, a definition quietly widened, prior methods placed in the wrong lineage or credited to the wrong work, a claim of novelty/universality the paper does not support, an invented citation. State that a single fabricated, misattributed, or over-broad claim caps this criterion near the bottom of its range no matter how fluent the rest is, and that vague attribution where a specific work is required is also a deduction.
   - Optionally one further craft criterion (<=0.15) such as judgment of emphasis (does the most important thing get the most space, and does the section give a specialist reader exactly the frame they need?) --- again with no content checklist.

4. Every criterion description must include an explicit "do not deduct for" clause naming what the grader must not punish (absent baselines, absent ablations, absent dataset or benchmark names, absent exact numbers, absent secondary mechanisms, absent extra prior-work themes, absent limitations sentence, implicit rather than announced positioning), and must state that additional correct detail earns zero extra credit.

5. Monotonicity test: no criterion may be more fully satisfied by adding material. If a criterion could be improved by pasting in one more fact from elsewhere in the paper, rewrite it.

6. Every criterion must be fully satisfiable in {target_words} words by a strong writer. If it could not be, cut it.

7. Forbid style tells as scoring bases: citation density or format, first person, section cross-references, presence or absence of numbers as such, paragraph count, or sentence-length uniformity.

8. Grading order, stated inside the descriptions: the grader must first ask "is anything here unnecessary, imprecise, over-claimed, or belonging to another section?" and only then ask "does the argument actually break for want of something?" Anchor full credit at "a competent expert wrote exactly what this section needs and stopped," and make clear that a clean, restrained, accurate section is a top-scoring section even if a more comprehensive candidate exists.

Output STRICT JSON only (no prose, no code fences) in exactly this shape:
{
  "criteria": [
    {"name": "<short name>", "description": "<what a grader checks, specific to this paper: what earns full credit and what to deduct for>", "weight": <float 0-1>}
    // 4 to 6 criteria; weights sum to 1.0
  ],
  "length_adherence": {"target_words": {target_words}, "tolerance": 0.15,
                        "note": "candidate should be within tolerance of target_words; do not reward extra length or extra detail"}
}

PAPER:
{paper}
\end{lstlisting}

\paragraph{Derived rubrics.} Applying this meta-prompt to a paper yields a
paper-specific rubric. We show three, generated by \textbf{Muse Spark} at
iteration~3. The first two are the \emph{same cell} (the abstract of \emph{Don't Waste
It}, a validation paper) under the blind and GT-informed variants---identical
instructions, different \texttt{\{paper\}} input---illustrating how ground-truth access
changes the generated criteria. The third is a blind related-work rubric on a second
paper.

\paragraph{Blind rubric --- \emph{Don't Waste It}, abstract.}
\begin{lstlisting}
{
  "criteria": [
    {
      "name": "Argument Integrity",
      "description": "Does the candidate deliver a coherent, self-sufficient version of what an abstract must do for THIS paper: a single arc from problem (accuracy-centric recommenders misaligned with broader human objectives) to limitation of status quo (post-hoc heuristics disconnected from representation learning, unsupervised E2E models as black boxes) to intervention (injecting structured human priors via lightweight prior-conditioned multi-head decoding) to payoff (accuracy plus better alignment on diversity/personalization/discovery with controllable disentangled representations), and is that claim true of ",
      "weight": 0.18
    },
    {
      "name": "Necessity and Scope Discipline",
      "description": "Is anything here material this section should not carry? For this paper, concrete over-inclusions that are liabilities in an abstract include: named datasets Pixel8M, MerRec, EB-NeRD; baseline set HSTU, HLLM, ComiRec, REMI, DualVAE; exact headline numbers Recall@5/10, NDCG@5/10, entropy H@K, 283,497 new-interest users; loss terms in-group negative sampling, frequency balancing w_freq, temporal discount gamma=0.7; optimizer/schedule; module names and equations SiLU residual adapter q_k = h_T + SiLU W^{(k)} h_T, zero-init, compatibility masking Omega_k, hierarchical composition tree Eq.5, max/av",
      "weight": 0.32
    },
    {
      "name": "Economy, Authorial Control, Non-Formulaic Prose",
      "description": "Reward sentences that are technically exact and subordinate detail to claims (main clause carries the point; specifics live in modifiers), varied paragraph shapes, transitions expressing real logical relations, and commitment instead of hedging. Penalize: restating the same contribution a second or third time, template scaffolding (thesis announced in sentence one, uniformly shaped paragraphs, paragraph-final 'however, this leaves a gap' clause, 'Moreover/Additionally/Furthermore' chains, 'Critically/Notably/Importantly' openers), hollow intensifiers ('significant', 'crucial', 'comprehensive',",
      "weight": 0.22
    },
    {
      "name": "Faithfulness, Attribution, Calibration",
      "description": "Check that claims are true of this paper and not over-broad. Concrete failure modes for this paper: attributing a gain number to the wrong backbone (HSTU vs HLLM) or configuration; describing the mechanism as cluster-then-encode or post-hoc filtering instead of the paper's encode-then-project with prior-conditioned residual adapters and compatibility masking; defining human priors to include unsupervised latent interests; placing multi-interest networks in VAE lineage or crediting disentanglement to wrong work; claiming novelty/universality the paper does not support (e.g., eliminates all post",
      "weight": 0.2
    },
    {
      "name": "Judgment of Emphasis",
      "description": "Does the most important thing get the most space, and does the section give a specialist reader exactly the frame they need? Reward centering the core idea (guiding generative recommenders with structured human priors via lightweight backbone-agnostic multi-head decoding yielding disentangled controllable representations) and its payoff beyond accuracy (diversity, personalization, interest discovery). Penalize spending majority of words on secondary instantiations (8 categories, 6 events, Leiden clusters, LT/ST splits), training tricks (in-group negatives, frequency balancing, gamma), or fusio",
      "weight": 0.08
    }
  ],
  "length_adherence": {
    "target_words": 220,
    "tolerance": 0.15
  }
}
\end{lstlisting}

\paragraph{GT-informed rubric --- same cell.}
\begin{lstlisting}
{
  "criteria": [
    {
      "name": "Argument integrity",
      "description": "Argument integrity for abstract: does candidate deliver one self-contained arc problem -> status-quo limitation -> what we do -> what it buys that is true of this paper, without requiring any particular fact list. Full credit if reader gets coherent, self-sufficient claim matching paper's actual contribution; any economical route to that argument earns full credit and a candidate selecting a different but coherent subset of material earns full credit. Deduct only if you can state in one sentence how absence makes argument false, unsupported, or incoherent; vague dissatisfaction like 'does not ",
      "weight": 0.18
    },
    {
      "name": "Necessity and scope discipline",
      "description": "Necessity and scope discipline - largest weight. Abstract must carry only what its job needs; baseline lists, dataset inventories, exact numbers, hyperparameters, architecture internals are liabilities. Concrete over-inclusions to treat as violations in this paper: naming Pixel8M/MerRec/EB-NeRD, listing HSTU/HLLM/ComiRec/REMI/DualVAE, enumerating Recall@5/10 NDCG@5/10 H@K or other headline numbers, detailing SiLU residual adapter equation q_k = h_T + SiLU(W h_T), compatibility masking Omega_k, hierarchical tree equations, frequency balancing w_freq, temporal discount gamma=0.7, max vs avg fusi",
      "weight": 0.32
    },
    {
      "name": "Economy and non-formulaic prose",
      "description": "Economy, authorial control, and non-formulaic prose. Full credit for sentences that are technically exact and subordinate detail to claims (main clause carries point, specifics in modifiers), varied paragraph shapes, transitions expressing real logical relations, commitment over hedging. Penalize restating same point second/third time, template scaffolding (opening thesis announcement 'In this paper we propose...', paragraph-final 'however this leaves a gap' declarations, Moreover/Additionally/Furthermore chains), hollow intensifiers (significant, crucial, comprehensive, state-of-the-art, grou",
      "weight": 0.2
    },
    {
      "name": "Faithfulness and calibration",
      "description": "Faithfulness, attribution, and calibration - strict. Check claims match paper: e.g., paper uses encode-then-project with lightweight prior-conditioned adapter heads on shared backbone, not cluster-then-encode or architecture-specific replacement; it reuses accumulated industrial human priors as strategic advantage, not inventing taxonomies; temporal discount optimum is 0.7 not RL-typical 0.9-0.995; diversity gain comes from prior-guided disentanglement not unsupervised discovery; hierarchical composition is sequential coarse-to-fine with shrinkage, not independent product heads. A single fabri",
      "weight": 0.2
    },
    {
      "name": "Judgment of emphasis",
      "description": "Judgment of emphasis. Does most important thing get most space and does specialist reader get exactly frame they need? For this paper central is turning accumulated post-hoc human priors into end-to-end training signal via backbone-agnostic lightweight heads that disentangle intent along interpretable axes, with hierarchical composition for interacting priors, yielding both accuracy and beyond-accuracy (diversity, personalization, discovery) and better scaling with context/size. Full credit when space allocation mirrors that: problem/gap and idea dominate, payoff stated without inventory. Pena",
      "weight": 0.1
    }
  ],
  "length_adherence": {
    "target_words": 220,
    "tolerance": 0.15
  }
}
\end{lstlisting}

\paragraph{Blind rubric --- Neuralangelo, related work.}
\begin{lstlisting}
{
  "criteria": [
    {
      "name": "Argument integrity for Related Work",
      "description": "Check whether the candidate makes a coherent, self-sufficient version of the job of Related Work in THIS paper: positioning prior work against this paper with correct, specific attribution, where positioning may be carried implicitly by precise technical description. An explicit gap paragraph is optional and manufactured themes are a defect. Grading order: first ask 'is anything here unnecessary, imprecise, over-claimed, or belonging to another section?' and only then ask 'does the argument actually break for want of something?' Full credit = a competent expert wrote exactly what this section ",
      "weight": 0.15
    },
    {
      "name": "Necessity and scope discipline",
      "description": "This is the largest criterion. Check whether every sentence is load-bearing for Related Work's job. In this paper, the following are liabilities and belong to other sections, not Related Work: named datasets DTU and Tanks and Temples, baseline set COLMAP/NeRF/VolSDF/NeuS/HF-NeuS/RegSDF/NeuralWarp/Geo-NeuS, exact headline numbers like Chamfer 0.61 or PSNR 33.84, loss terms L_RGB/L_eik/L_curv and weights w_eik=0.1/w_curv, optimizer/schedule AdamW/500k iterations/lr 1e-3/warmup/decay, module names SDF MLP 1-layer/color MLP 4-layer/hash resolutions 2^5 to 2^11/16 levels/2^22 entries/channel 8, abl",
      "weight": 0.35
    },
    {
      "name": "Economy, authorial control, non-formulaic prose",
      "description": "Check whether sentences are technically exact and subordinate detail to claims (main clause carries point; specifics live in modifiers), with varied paragraph shapes and transitions expressing real logical relations, and commitment instead of hedging. Penalize: restating same point a second or third time, template scaffolding like thesis announcement in sentence one, uniformly shaped paragraphs each closing with 'however, this leaves a gap', chains of Moreover/Additionally/Furthermore, hollow intensifiers 'significant/crucial/comprehensive/state-of-the-art', promotional framing, vacuous opener",
      "weight": 0.2
    },
    {
      "name": "Faithfulness, attribution, and calibration",
      "description": "Check for precise, calibrated attribution specific to this paper. Concrete failure modes to watch for: describing numerical gradients as replacing analytical gradients for RGB rendering instead of for eikonal/curvature regularization to smooth hash-grid normals; claiming hash encoding uses hierarchical octree spatial decomposition like sparse voxels when paper says it assumes no hierarchy and resolves collisions by gradient averaging; attributing Instant NGP to wrong lineage or conflating NeuS SDF volume rendering Eq 3 with VolSDF density conversion; claiming Neuralangelo requires depth/segmen",
      "weight": 0.2
    },
    {
      "name": "Judgment of emphasis",
      "description": "Check whether the most important positioning gets the most space and whether a specialist reader gets exactly the frame they need, without manufactured themes or equal-weight laundry lists. Reward selective emphasis that lets core lineage (neural surface rendering vs hash encoding scalability) dominate and secondary threads stay subordinate. Penalize giving equal space to tangential lineages or inflating minor points to fill length. Grading order: first ask 'is anything here unnecessary, imprecise, over-claimed, or belonging to another section?' and only then ask 'does the argument break for w",
      "weight": 0.1
    }
  ],
  "length_adherence": {
    "target_words": 505,
    "tolerance": 0.15
  }
}
\end{lstlisting}
